# Supplementary material for: PairBench: Are Vision-Language Models Reliable at Comparing What They See?
Source: arXiv:2502.15210 source file (2025-05-29)
Supplement: Supplementary file 1 [file 86_human_study.tex]

% \subsection{Human Study for Ground Truth Scores}
% \label{sec:human-study}

% \begin{table}[ht]
% \centering
% \caption{Human similarity scores (mean ± std) across different transformation settings, which we used to set our ground truth scores.}
% \resizebox{\linewidth}{!}{%
% \begin{tabular}{lcc|cc|cc}
% \toprule
% \textbf{Pair Type} 
% & \multicolumn{2}{c|}{\textbf{Colorjitter}} 
% & \multicolumn{2}{c|}{\textbf{Perspective}} 
% & \multicolumn{2}{c}{\textbf{Rotate}} \\
% & \textbf{Sens} & \textbf{Invar} 
% & \textbf{Sens} & \textbf{Invar} 
% & \textbf{Sens} & \textbf{Invar} \\
% \midrule
% Identical   & 9.8 ± 0.53  & 9.95 ± 0.23  & 9.82 ± 0.42  & 9.9 ± 0.32   & 10.0 ± 0.0   & 9.89 ± 0.51 \\
% Transformed & 5.5 ± 2.3   & 9.68 ± 0.85  & 6.89 ± 1.97  & 9.06 ± 1.33  & 6.31 ± 2.01  & 9.36 ± 1.01 \\
% Irrelevant  & 1.35 ± 0.74 & 1.42 ± 0.67  & 1.33 ± 0.81  & 1.61 ± 1.17  & 1.27 ± 0.64  & 1.23 ± 0.47 \\
% \bottomrule
% \end{tabular}
% }
% \end{table}
